# Supplementary material for: Giant thermovoltage in single InAs-nanowire field-effect transistors
Source: arXiv:1312.2835 source file (2013-12-10)
Supplement: Supplementary file 1 [file Roddaro_130423_SM.pdf]

# SUPPLEMENTARY MATERIAL: Giant thermovoltage in single InAs nanowire field-effect transistors

Stefano Roddaro,[1,2,*] Daniele Ercolani,[1] Mian Akif Safeen,[1] Soile Suomalainen,[3]
Francesco Rossella,[1] Francesco Giazotto,[1] Lucia Sorba,[1] and Fabio Beltram[1]

[1]*NEST, Scuola Normale Superiore and Istituto Nanoscienze-CNR, Piazza S. Silvestro 12, I-56127 Pisa, Italy*
[2]*Istituto Officina dei Materiali – CNR, Basovizza S.S. 14 km 163.5, I-34149 Trieste, Italy*
[3]*Optoelectronics Research Centre, Tampere University of Technology, P.O. Box 692, FIN-33101 Tampere, Finland*

PACS numbers: 72.20.Pa, 81.07.Gf, 85.30.Tv

## I. HEATER OPERATION

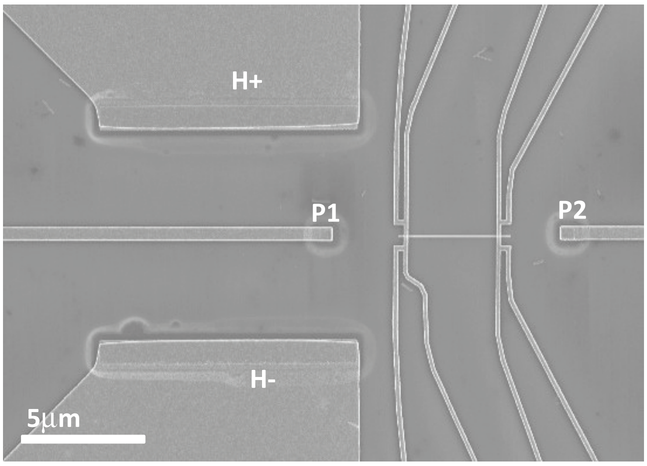


FIG. 1: Top view one of the measured devices. The current injection contacts of the buried heater are marked as $H\pm$ and are used to induce a graded current density in the Si substrate. Two probe contacts $P1$ and $P2$ are used to measure the actual substrate potential below the nanowire, in order to detect small deviations from the average $(V_{H+} + V_{H-})/2$ which would be expected by symmetry in the case of ideal contacts.

In the thermal biasing experiments, two voltages $V_{H\pm} = V_0 \pm V_H$ were fed into the $H\pm$ contacts. This induced gating by the substrate $V_{bg} \approx (V_{H+}+V_{H-})/2 = V_0$ and a thermal gradient at the NW position. Despite the symmetry of the device structure, the precise value of the backgate is hard to predict due to the non-ideal behavior of the metal-semiconductor interfaces at the injection contacts $H_\pm$. For this reason, two voltage probes $P_1$ and $P_2$ (see Fig. 1) were used to directly *measure* the actual backgate potential $V_{bg}$. The voltage difference between the two was typically found to be of the order of 1 mV thus assuring that sufficiently uniform gating was achieved below the NW position. A typical deviation of $\approx 0.2 - 0.4$ V was observed between $V_0$ and $V_{bg}$, most probably as a consequence of non-linear effects between the two $H\pm$ contacts and of differences between their resistances. The maximum gradient obtained during the experiment was $\approx 5\,\mathrm{K}/\mu\mathrm{m}$ with $V_H = 1.85$ V and $I_H \approx 90 - 100$ mA (depending on bath temperature). This was thus obtained with a power of $\approx 350$ mW and small overall average heating above the bath temperature of few tens of degree. This good performance was obtained thanks to the careful design of the injection contacts $H+$ and $H-$, which in turn determine the current distribution and position-dependent Joule heating in the bulk Si substrate. The detailed principle of operation and performance of our buried heater as a function of $V_H$ are not relevant to the NW analysis described here and go beyond the scope of the present paper: they will be thus discussed elsewhere.

## II. THERMAL AND ELECTRICAL CALIBRATIONS

The temperature at the two contacts $S$ and $D$ of the NWs were determined using four-wire Ti/Au resistive thermometers. Differential resistance of the $S$ and $D$ contacts was determined using an AC current of $\approx 5\,\mu A$ at 165 Hz

and 175 Hz by applying a 0.5 V excitation through a 100 kΩ biasing resistor plus a decupling capacitor. The voltage probes $V_{S\pm}$ and $V_{D\pm}$ were connected to two different AC-coupled lock-ins and calibrated against the reading of a factory-calibrated Si-diode thermometer. A simultaneous two-wire DC measurement yielded the electrical current $I_{DS}$ flowing through the NW at different electrical- and thermal-bias conditions. In order to avoid spurious effects due to thermal cycling[1], thermometers were calibrated by slowly changing (over $\approx 1$ hour) the overall temperature of the device in a $\Delta T \approx 60 - 100$ K range around the bath temperature (see Fig. 2a) before every heating sequence. Similarly, the current and voltage offsets were carefully nulled based on the fixed point of the IV characteristics of the NW as a function of the back-gate voltage $V_{bg}$ and at $\Delta T = 0$. These calibrations were performed after each variation of the bath temperature and, subsequently, a set of measurements were performed for different heater biases $V_H$, i.e. for different heater powers. This procedure was established in order to minimize the known history issues of the resistive thermometers. As an example, we report in Fig. 2b the extracted $V_{th}$ values for a bath temperature of $\approx 293$ K and $V_H = 0.5$ V (13 mA and 7 mW), 1 V (40 mA and 40 mW), 1.5 V (71 mA and 107 mW) and 1.85 V (96 mA and 178 mW). By powering the heater we obtain a thermal bias $\Delta T = 0.42$, 2.51, 6.87 and 11.71 K. The corresponding Seebeck values as a function of the resistance $R$ are reported in Fig.2c. The minor shift and discrepancy between the curves are due to the increased average temperature $T = (T_S + T_D)/2$ caused by the heater operation at larger and larger values of $V_H$. Differently, an even clearer consistency between the datasets is highlighted in Fig. 2d where we report $S/T$ which is weakly dependent on temperature. We note that data at high resistance are more scattered and imprecise, despite the large values of $V_{th}$ and $S$. This is a consequence of our parameter-extraction procedure, based on the analysis of the IV characteristics, which was adopted in order to extract both $S$ and $R$ as a function of the backgate voltage $V_{bg}$. The voltage intercept estimate is in fact less precise in the high-resistance limit and was in the present set-up implementation affected by the small AC current bias in the $S$ and $D$ leads. A direct open-circuit measurement of $V_{th}$ yielded an improved (and consistent) result but did not allow the simultaneous evaluation of $R$. Consequently, it was performed only to cross-check in a limited set of thermal-bias configurations.

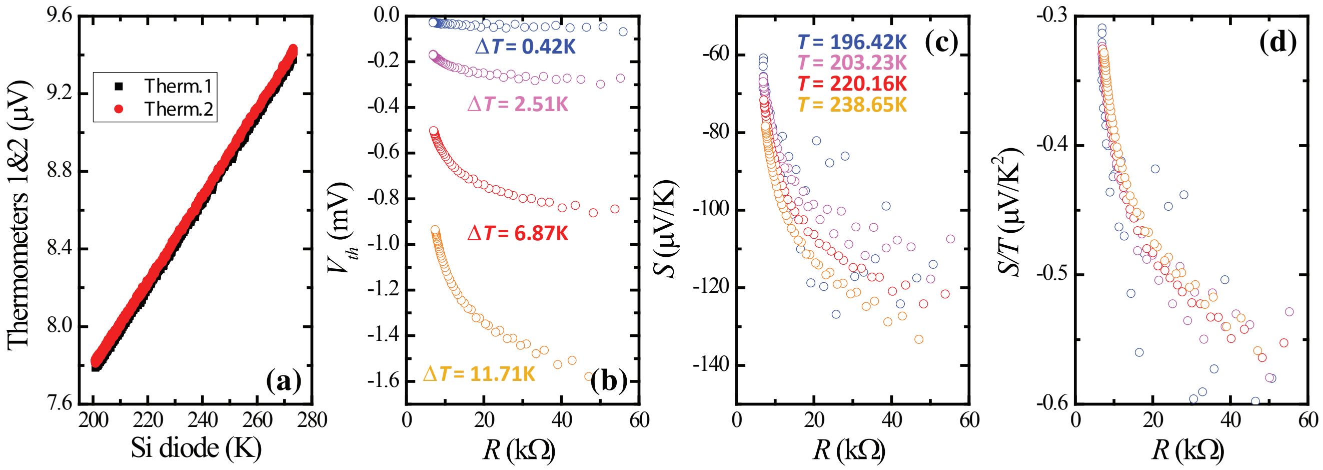


FIG. 2: (a) Calibration of the two thermometers in the range 200 − 280 K. An almost perfectly linear dependence was typically observed even over relatively large temperature intervals. Minor slope variations were observed as a function of the temperature and, most importantly, after thermal cycling: all these effects were taken into account by performing similar calibrations after each variation of the bath temperature. (b) Thermovoltage $V_{th}$ versus resistance $R$ curves obtained for different heater biasing of $V_H = 0.5$, 1.0, 1.5 and 1.85 V and corresponding Seebeck coefficient (panel (c)). The difference between the curves is merely due to the average increase in the nanowire temperature $T = (T_S + T_D)/2$, as visible in the consistent plot $S/T$ in panel (d).

## III. ESTIMATE OF THE FIELD-EFFECT MOBILITY $\mu_{e,FE}$

Carrier density and mobility in the NW FETs were calculated using a standard charge-control method, based on the device transconductance and on an estimate of the capacitance between the NW body and the back-gate electrodes. The simple model allows to estimate the mobility following

$$\mu_{e,FE} = \frac{L^2}{C_{bg}} \frac{dG}{dV_{bg}}. \tag{1}$$

The precise value of $C_{bg}/L$ was numerically calculated using the partial differential equation solver COMSOL and found to be equal to 41 aF/$\mu$m (see Fig. 3a). This value is in good agreement with standard numerical estimates in agreement with approximate analytical models[2]. The mobility estimate for the datasets reported in our paper are shown in Fig. 3b for $T = 116.6$, 155.0, 195.9 and 238.6 K. Curves were obtained by changing the gate voltage as a speed of $\approx 1$ V/min from positive towards negative values. Even if the model can be considered to be strictly valid only when $\partial\mu_e/\partial V_{bg} = 0$, i.e. at peak mobility, the estimate $\mu_{e,FE}$ was found to be undoubtedly and significantly lower than one obtained using the Seebeck effect ($\mu_e \gtrsim 10000\,\mathrm{cm}^2$/Vs). This result is in agreement with recent experimental results suggesting a systematic underestimate of the carrier mobility in a standard field-effect approach owing to screening by trap charges. Indeed, despite the slow sweeping speed, gate hysteresis was observed even at $T \approx 100$ K and different $\mu_{e,FE}$ peak values could be extracted. A slightly larger mobility was estimated from gate sweeps from the pinch-off towards positive values of $V_{bg}$ but none of the estimates ever exceeded $5000\,\mathrm{cm}^2$/Vs in any of the studied configurations.

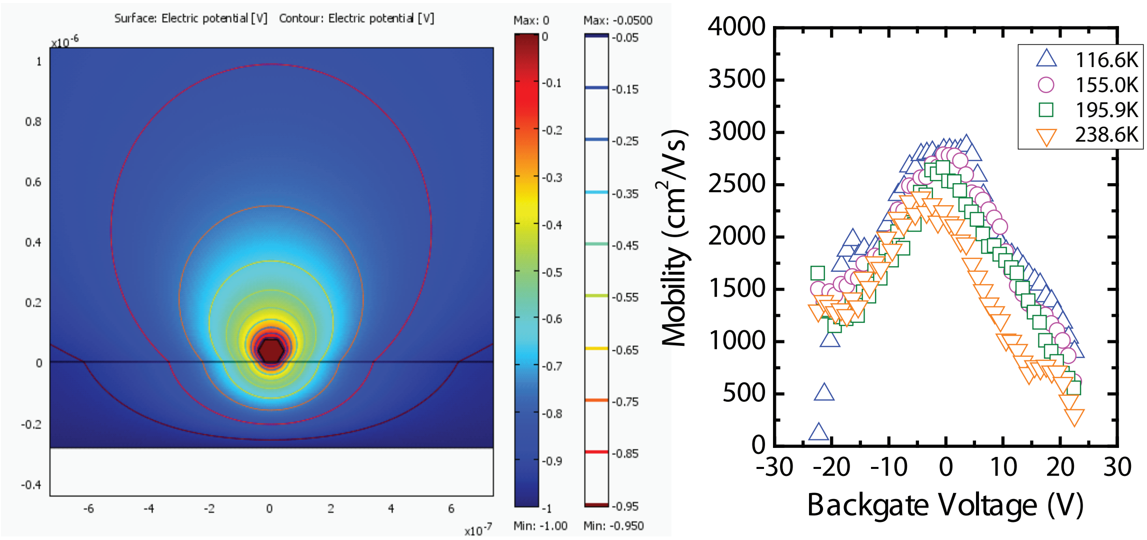


FIG. 3: (a) Electrostatic simulation of the field effect on a 73 nm-diameter NW in the case of a 280 nm $SiO_2$ oxide. The nanowire was modeled as a metallic hexagonal conductor and quantum capacitance effects were neglected as they are known to provide only a marginal correction for InAs nanowires of this size. The backgate was set to $-1$ V and the potential variation and equipotential lines are visible in the colorplot. The estimated capacitance per unit length was 41 aF/$\mu$m. (b) Calculated carrier mobility: a mild monotonic increase is observed on lowering the sample temperature, within the explored range.

* Electronic address: s.roddaro@sns.it

[1] Q. Cai, Y.-C. Chen, C. Tsai, J. F. De Natale *Development of a platinum resistance thermometer on the silicon substrate for phase change studies*, J. Micromech. Microeng. **22**, 085012 (2012).
[2] O. Wunnicke, *Gate capacitance of back-gated nanowire field-effect transistors*, Appl. Phys. Lett. **89**, 083102 (2006).
